# Supplementary material for: ImDrug: A Benchmark for Deep Imbalanced Learning in AI-aided Drug Discovery
Source: arXiv:2209.07921 source file (2022-10-18)
Supplement: Supplementary file 2 [file Appendix-H-Revision.tex]

\section{Revision of Fig.~\ref{fig:compare} in the Main Text}
We are sorry that there exists a minor mistake in Fig.~\ref{fig:compare} of Sec.~\ref{sec:4.1} in the main text (we mistakenly used the same data to draw both plots of balanced f1 and AUROC). We hereby declare that we make a revision of Fig.~\ref{fig:compare1} in this section, which is reflected in the main text of this version of manuscript.

\begin{figure}[h]
    \centering
    \includegraphics[width=0.92\textwidth]{Figures/compare.pdf}
    \caption{\textbf{Comparison of the baseline performance for standard and random splits} on USPTO-50K, in terms of balanced accuracy, balanced F1 and AUROC. The 2 proposed balanced metrics exhibit a good Pearson's R correlation between the two splits (0.7466, 0.7353), which is significantly higher than AUROC (0.6580).}
    \label{fig:compare1}
\end{figure}
