# Supplementary material for: ImDrug: A Benchmark for Deep Imbalanced Learning in AI-aided Drug Discovery
Source: arXiv:2209.07921 source file (2022-10-18)
Supplement: Supplementary file 3 [file Appendix-I-Limitations.tex]

\section{Limitations}
\label{sec:limitations}
